# Supplementary material for: Towards Models that Can See and Read
Source: arXiv:2301.07389 source file (2023-03-21)
Supplement: Supplementary file 1 [file appendix_main.tex]

% % CVPR 2023 Paper Template
% % based on the CVPR template provided by Ming-Ming Cheng (https://github.com/MCG-NKU/CVPR_Template)
% % modified and extended by Stefan Roth (stefan.roth@NOSPAMtu-darmstadt.de)

% \documentclass[10pt,twocolumn,letterpaper]{article}

% %%%%%%%%% PAPER TYPE  - PLEASE UPDATE FOR FINAL VERSION
% % \usepackage[review]{cvpr}      % To produce the REVIEW version
% \usepackage{cvpr}              % To produce the CAMERA-READY version
% %\usepackage[pagenumbers]{cvpr} % To force page numbers, e.g. for an arXiv version

% % Include other packages here, before hyperref.
% \usepackage{graphicx}
% \usepackage{amsmath}
% \usepackage{amssymb}
% \usepackage{booktabs}
% \usepackage{pifont}
% \usepackage{multirow}
% \usepackage{arydshln}
% \usepackage[outercaption]{sidecap}    
% \usepackage{color, colortbl}
% \usepackage[dvipsnames]{xcolor}
% \usepackage[title]{appendix}
% \usepackage{enumitem}
% \usepackage{bm}
% \definecolor{LightGray}{rgb}{0.92,0.92,0.92}
% \definecolor{Red}{rgb}{1.0, 0.13, 0.32}
% \usepackage{tikz}
% \usepackage{arydshln}
% \usepackage{subcaption}
% \usepackage{adjustbox}
% \usepackage{wrapfig}
% \newcommand{\zyang}[1]{{\color[rgb]{0,0,1}{\tiny\textbf{ZY:}}{\normalsize\itshape#1}}}
% \newcommand{\eat}[1]{}
% % It is strongly recommended to use hyperref, especially for the review version.
% % hyperref with option pagebackref eases the reviewers' job.
% % Please disable hyperref *only* if you encounter grave issues, e.g. with the
% % file validation for the camera-ready version.
% %
% % If you comment hyperref and then uncomment it, you should delete
% % ReviewTempalte.aux before re-running LaTeX.
% % (Or just hit 'q' on the first LaTeX run, let it finish, and you
% %  should be clear).
% \usepackage[pagebackref,breaklinks,colorlinks]{hyperref}


% % Support for easy cross-referencing
% \usepackage[capitalize]{cleveref}
% \crefname{section}{Sec.}{Secs.}
% \Crefname{section}{Section}{Sections}
% \Crefname{table}{Table}{Tables}
% \crefname{table}{Tab.}{Tabs.}

% \input{math_commands}


% %%%%%%%%% PAPER ID  - PLEASE UPDATE
% \def\cvprPaperID{2817} % *** Enter the CVPR Paper ID here
% \def\confName{CVPR}
% \def\confYear{2023}

% \newcommand{\ganz}[1]{{\color{red} [ganz: #1]}}
% \newcommand\aviadsuggestion[1]{\textcolor{blue}{\textit{aviad}: #1}}
% % \def\checkmark{\tikz\fill[scale=0.4](0,.35) -- (.25,0) -- (1,.7) -- (.25,.15) -- cycle;} 


% \begin{document}

% %%%%%%%%% TITLE - PLEASE UPDATE
% \title{Towards Models that Can See and Read}

% \author{
% Roy Ganz\thanks{Work done during an Amazon internship.}\\
% Technion, Israel\\
% {\tt\small ganz@cs.technion.ac.il}
% \and
% Oren Nuriel\\
% AWS AI Labs\\
% {\tt\small \{onuriel\}@amazon.com}
% \and
% Aviad Aberdam\\
% AWS AI Labs\\
% {\tt\small aaberdam@amazon.com}
% \and
% Yair Kittenplon\\
% AWS AI Labs\\
% {\tt\small yairk@amazon.com}
% \and
% Shai Mazor\\
% AWS AI Labs\\
% {\tt\small \{smazor\}@amazon.com}
% \and
% Ron Litman\\
% AWS AI Labs\\
% {\tt\small \{litmanr\}@amazon.com}
% }
% \maketitle

% \newcommand{\AlgoName}{UniTNT }
% \newcommand{\AlgoNameNoSpace}{UniTNT}
% \newcommand{\AlgoNameBLIP}{UniTNT-BLIP }
% \newcommand{\AlgoNameNoSpaceBLIP}{UniTNT-BLIP}
% \newcommand{\AlgoNameOFA}{UniTNT-OFA }
% \newcommand{\AlgoNameNoSpaceOFA}{UniTNT-OFA}

% %******************

% \appendix
% \input{appendix_content}

% \clearpage

% %%%%%%%%% REFERENCES
% {\small
% \bibliographystyle{ieee_fullname}
% \bibliography{egbib}
% }

% \end{document}
